# Supplementary material for: Limitations of coupled cluster approximations for highlyaccurate investigations of Rb$_2^+$
Source: arXiv:2107.00103 ancillary file (2021-06-30)
Supplement: Supplementary file 1 [file Supplementary_paper_rb2plus.pdf]

# Supplementary Material: Limitations of coupled cluster approximations for highly accurate investigations of $Rb_2^+$

Jan Schnabel,[1] Lan Cheng,[2] and Andreas Köhn[1]
[1)]*Institute for Theoretical Chemistry, University of Stuttgart, Pfaffenwaldring 55, D-70569 Stuttgart, Germany*
[2)]*Department of Chemistry, The Johns Hopkins University, Baltimore, Maryland 21218, United States*

(*Electronic mail: schnabel@theochem.uni-stuttgart.de)

(*Electronic mail: lcheng24@jhu.edu)

(*Electronic mail: koehn@theochem.uni-stuttgart.de)

## I. INVESTIGATING THE INDEPENDENCE OF THE LONG-RANGE HUMP ON POSSIBLE SOURCES OF ERROR

In the main text we claimed that the unphysical long-range barrier of the $X\,^2\Sigma_g^+$ PEC of $Rb_2^+$ is independent on a number of possible sources of error. In the following we will support this statement by showing the corresponding graphs.

### A. Tightened convergence thresholds

We exclude numerical errors due to convergence issues since we tightened the thresholds in all of our computations as follows:

1. MOLPRO:
   - RHF reference calculation uses threshold `accu=14`
   - UCCSD(T) calculation uses `thrden=1.d-12` and `thrvar=1.d-16`
2. CFOUR:
   - `SCF_CONV=11` and `CC_CONV=11`

### B. Basis-set superposition error

As mentioned in the main text we checked for basis-set superposition errors (BSSEs) by applying the counterpoise correction (cpc) scheme. Aside from the fact that this possible source of error in small systems as $Rb_2^+$ is more conveniently suppressed by using rather large basis-sets, Fig. S1 illustrates that the long-range barrier is not due to BSSEs. Moreover, we note that accounting for BSSEs or not is quite a small effect in the long-range region as shown by the energy differences in Fig. S1 (b).

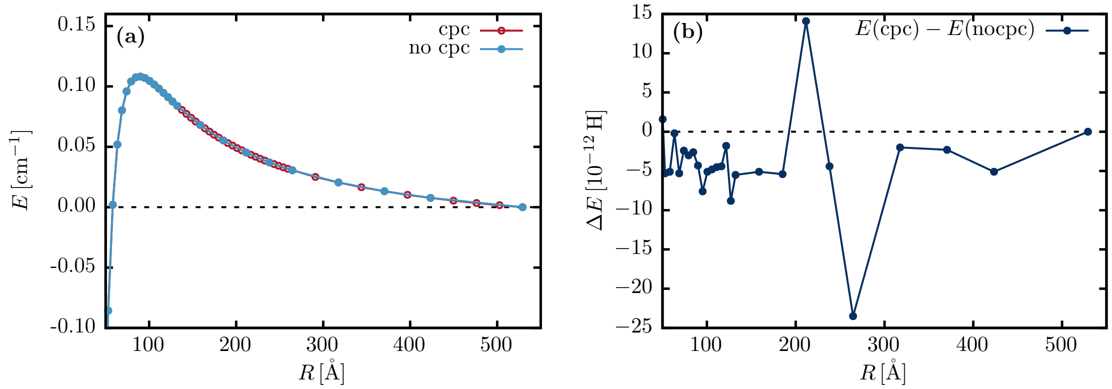


Figure S1. Comparison of RHF-UCCSD/ECP28MDF/aug-cc-pCVTZ-PP results obtained by applying the counterpoise correction (cpc) scheme and without counterpoise correction (nocpc). The long-range tail of the $X\,^2\Sigma_g^+$ PEC in **(a)** shows that the breakdown of CCSD(T) is not just an artefact of basis set superposition errors (BSSEs). The difference between both PECs, depicted in **(b)**, demonstrates that this effect is rather small in the long-range region.

## C. RHF-RCCSD(T) versus RHF-UCCSD(T)

In Fig. S2 we show that the unphysical long-range barrier occurs both for the partially spin-restricted [RHF-RCCSD(T)] and the spin-unrestricted [RHF-UCCSD(T)] variant of MOLPRO's coupled-cluster implementations. The difference in the resulting interaction energies is shown in Fig. S2 (b).

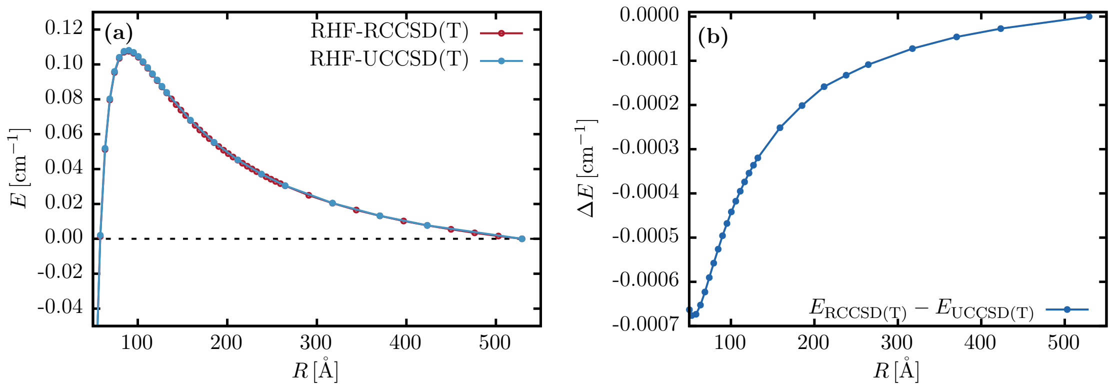


Figure S2. **(a)** The long-range part of the $Rb_2^+$ ground state PEC using either the partially spin-restricted variant of coupled-cluster theory [RHF-RCCSD(T)] or the spin-unrestricted one [RHF-UCCSD(T)]. Both methods are implemented in the MOLPRO program package. Both calculations are based on the ECP28MDF pseudo-potential and the aug-cc-pCVTZ-PP basis set. The difference in the interaction energies of both methods is shown in **(b)**.

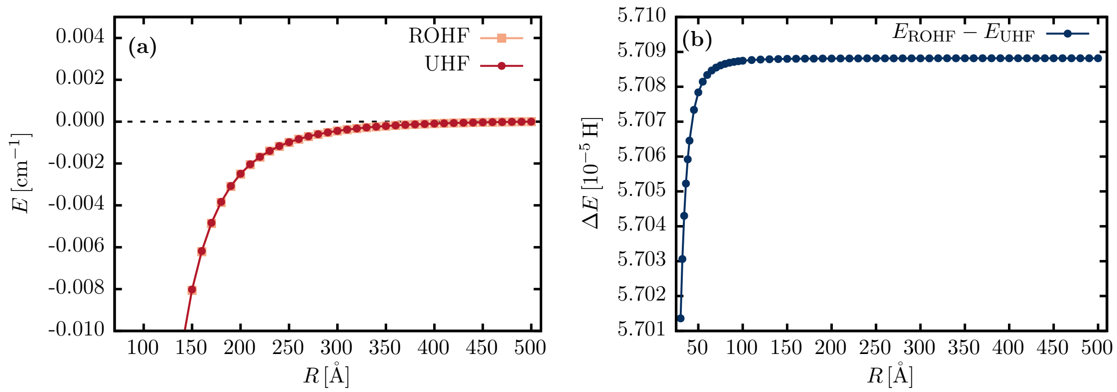


Figure S3. Difference between ROHF and UHF reference wavefunctions for computing the ground state PEC of $Rb_2^+$. **(a)** Shows the corresponding interaction energies calculated relative to the last *ab-initio* points. ROHF energies were computed with the MOLPRO program package while UHF-energies resulting from CFOUR calculations. Differences between ROHF and UHF (absolute) reference energies shown in **(b)** are in the order of $\mathcal{O}(10^{-5}\,\mathrm{H})$. The calculations correspond to ECP28MDF/aug-cc-pCVTZ-PP level of theory.

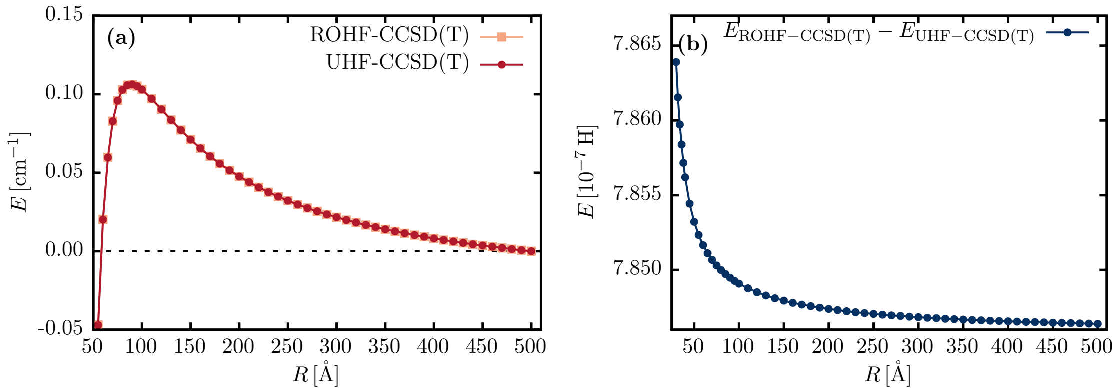


Figure S4. Comparison of the impact of using different reference wavefunctions for the subsequent coupled-cluster calculations. The long-range $X\,^2\Sigma_g^+$ PECs shown in**(a)** demonstrate that the unphysical barrier is independent on the choice of the reference wavefunction. In **(b)** it is shown that an restricted or unrestricted open-shell reference ansatz does not matter much in the coupled-cluster calculations. The difference between both approaches is in the order of $\mathcal{O}(10^{-7}\,\mathrm{H})$. The calculations were performed using ECP28MDF/aug-cc-pCVTZ-PP level of theory.

## D. The choice of the reference wavefunction

In Fig. S3 we investigate the ground state PEC of $Rb_2^+$ at Hartree-Fock level of theory using different approaches. The energy difference (in terms of absolute energies) between UHF and ROHF wavefunctions is in the order of $\mathcal{O}(10^{-5}\,\mathrm{H})$ as shown in Fig. S3 (b). However, independent on the choice of the reference wavefunction, we obtain the same unphysical long-range barrier for the subsequent CCSD(T) calculations. This is illustrated in Fig. S4. As MOLPRO does not support coupled-cluster methods based on UHF orbitals, the corresponding calculations have been performed using the CFOUR program package. Figure. S4 (b)

shows that an restricted or unrestricted open-shell reference ansatz does not matter much in the subsequent coupled-cluster calculations with energy differences in the order of $\mathscr{O}(10^{-7}\,\mathrm{H})$.

## II. UNIVERSAL PROBLEM FOR $X_2{}^+$- SYSTEMS

The unphysical barrier, which is discussed in detail in the main text, turns out to be universal for $X_2{}^+$– systems (with X = Li,Na, K, Rb, Cs), using iterative and non-iterative coupled cluster methods. This is shown in Fig. S5 for RHF-UCCSD(T) calculations. At this, no ECP has been used for Li and Na computations, while we used ECP10MDF for K and ECP46MDF for Cs.

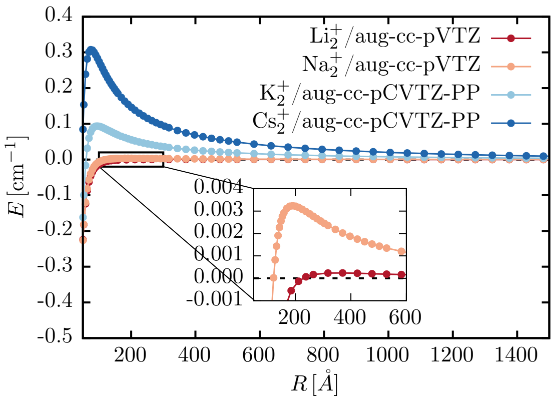


Figure S5. Long-range region of the PECs of several alkali-dimer cations. Calculations have been performed using the RHF-UCCSD(T) method leading to an unphysical long-range barrier for every species.

## III. MORE DETAILS ON SYMMETRY BREAKING

In the main text we pointed out that symmetry broken solutions suddenly collapse to the symmetry-adapted ones. In the following we investigate this in more detail. We found that the symmetry broken and symmetry-adapted solutions coincide for $R < R_{\mathrm{CF}} \approx 12.6\,\AA$. Beyond this so-called Coulson-Fischer point the symmetry-broken solution branches off the symmetric one with an discontinuous derivative at $R = R_{\mathrm{CF}}$. This first happens for ROHF results but also for ROHF-CCSD and ROHF-CCSD(T) as shown on the left-hand side of Fig. S6. Deeper insights are obtained by investigating the corresponding energy differences as demonstrated on the right-hand side of Fig. S6. First, we note that all symmetry-broken solutions decay slightly faster to the equilibrium state than the symmetry-adapted solutions do. This becomes noticeable in terms of a tiny hump in the difference curves. For ROHF-CCSD(T) results this effect is amplified by the long range hump which is the key point of this work. Moreover, for ROHF-CCSD and ROHF-CCSD(T) PECs there is a trough for $R \in [R_{\mathrm{CF}}, 15\,\AA]$. In case of the ROHF-CCSD solutions this is due to an intersection between symmetry broken and non-broken curves behind the Coulson-Fischer point. For ROHF-CCSD(T) PECs this trough is much more pronounced due to an additional hump in the symmetry-broken solution shown by the lower inset in Fig. S6 (e).

The origin of this additional hump becomes clear when also considering the $\Sigma_u$ PEC. This is shown in Fig. S7. Due to the numerical bistability of the symmetry broken solution it shows strong mixings with the $\Sigma_u$

state, which, for $C_{2v}$ calculations, falls into the same IRREP as the $\Sigma_g$ state, in the above mentioned region (i.e. $R \in [R_{\mathrm{CF}}, 15\,\text{Å}]$). This also somehow marks the transition between short range and long range. In other words, in this transition, or intermediate region the symmetry-broken solution cannot "decide" between the $\Sigma_g$ and $\Sigma_u$ states which are degenerate in the long range. This is furthermore demonstrated by the energy differences in Fig. S7 (b) where the difference $\Sigma_u(D_{2h}) - \Sigma_g(C_{2v})$ approaches zero in this region.

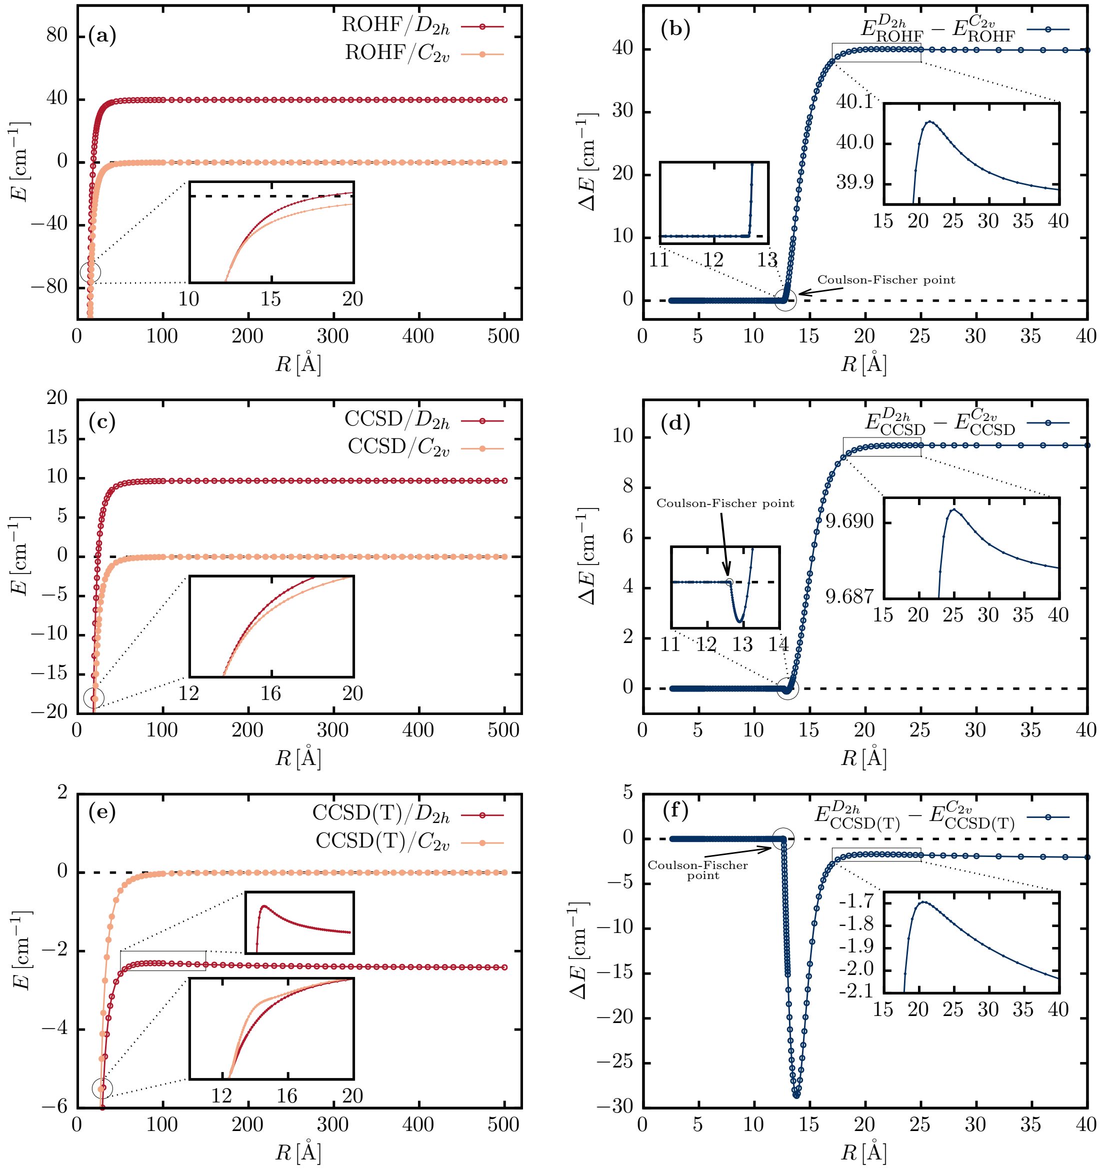


Figure S6. Comparison of symmetry broken and non-broken ROHF, ROHF-CCSD and ROHF-CCSD(T) solutions obtained at ECP28MDF/aug-cc-pCVTZ-PP level of theory. The **upper panel** shows the ROHF-PECs relative to the separated fragments, i.e. Rb+Rb$^+$ in **(a)**. The inset shows that at a critical internuclear separation $R_{\mathrm{CF}}$ – the Coulson-Fischer point – the symmetry broken solution branches off from the symmetry adapted one. This is highlighted in **(b)** by the corresponding energy differences. The inset on the right-hand side indicates that the symmetry broken solution decays slightly faster to the equilibrium state than the symmetry-adapted one. The inset on the left-hand side depicts the vicinity of the Coulson-Fischer point. Accordingly the same is shown in the **middle panel** in **(c)** and **(d)** for ROHF-CCSD PECs and in the **lower panel** in **(e)** and **(f)** for ROHF-CCSD(T) results. Here, the small hump of the symmetry-broken solution shown in the lower inset in **(e)** is discussed in the text and in Fig. S7.

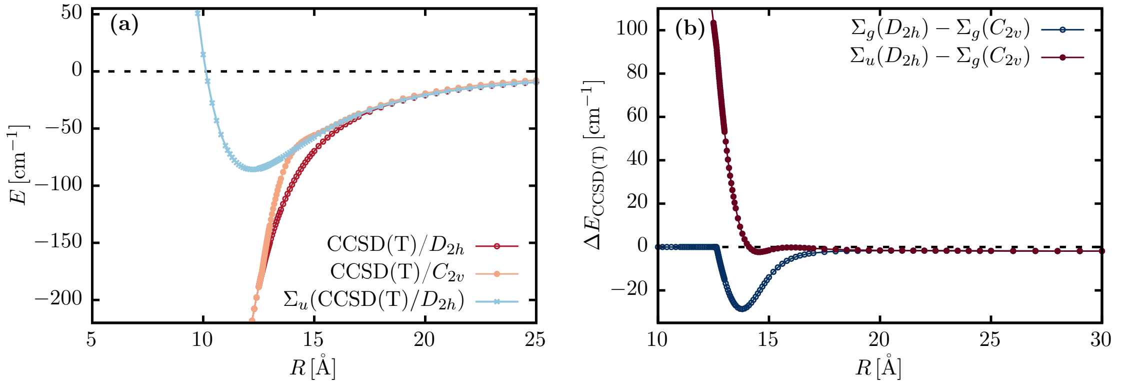


Figure S7. Close-up of the ROHF-CCSD(T) symmetry-broken and symmetry-adapted solutions for the ground state PECs of the $\Sigma_g$ state together with the (symmetry-adapted) $\Sigma_u$ PEC. The energies in **(a)** are given relative to the separated fragments (i.e. Rb+$Rb^+$) and are calculated at ECP28MDF/aug-cc-pCVTZ-PP level of theory. The small hump in the symmetry-broken ROHF-CCSD(T) solution of the $\Sigma_g$ state is due to the numerical bistability yielding an area with mixing to the $\Sigma_u$ state which, for $C_{2v}$ calculations, falls into the same IRREP. This is also shown by the energy differences in **(b)** where in the region of the hump the difference to the $\Sigma_u$ state is close to zero.
